# Supplementary material for: Complex pressure-temperature structural phase diagram of honeycomb iridate Cu$_2$IrO$_3$
Source: arXiv:2105.01122 ancillary file (2021-05-03)
Supplement: Supplementary file 1 [file supplemental.pdf]

# Supplementary Material: Complex pressure-temperature structural phase diagram of honeycomb iridate $\text{Cu}_2\text{IrO}_3$

G. Fabbri,<sup>1,\*</sup> A. Thorn,<sup>2</sup> W. Bi,<sup>1,3,4</sup> M. Abramchuk,<sup>5</sup> F. Bahrami,<sup>5</sup> J. H. Kim,<sup>1</sup> T. Shinmei,<sup>6</sup> T. Irifune,<sup>6,7</sup> F. Tafti,<sup>5</sup> A. N. Kolmogorov,<sup>2</sup> and D. Haskel<sup>1</sup>

<sup>1</sup>*Advanced Photon Source, Argonne National Laboratory, Argonne, Illinois 60439, USA*

<sup>2</sup>*Department of Physics, Applied Physics and Astronomy,  
Binghamton University, State University of New York,  
PO Box 6000, Binghamton, New York 13902-6000, USA*

<sup>3</sup>*Department of Geology, University of Illinois at Urbana-Champaign, Urbana, Illinois 61801, USA*

<sup>4</sup>*Department of Physics, University of Alabama at Birmingham, Birmingham, AL 35294, USA*

<sup>5</sup>*Physics Department, Boston College, Chestnut Hill, Massachusetts 02467, USA*

<sup>6</sup>*Geodynamics Research Center, Ehime University, Matsuyama, 790-8577, Japan*

<sup>7</sup>*Earth-Life Science Institute, Tokyo Institute of Technology, Tokyo, Japan*

(Dated: April 23, 2021)

|      |                                                                                                      |    |
|------|------------------------------------------------------------------------------------------------------|----|
| I    | Further details on the powder x-ray diffraction analysis .....                                       | 2  |
| II   | Additional x-ray absorption fine structure information .....                                         | 2  |
| III  | Table S1 Experimental lattice constants .....                                                        | 2  |
| IV   | Table S2 Experimental and theoretical atomic positions at 1 bar .....                                | 3  |
| V    | Table S3 Theoretical atomic positions at 10 GPa.....                                                 | 3  |
| VI   | Table S4 Theoretical atomic positions at 25 GPa.....                                                 | 3  |
| VII  | Figure S1 Experimental PXRD data and Rietveld refinements .....                                      | 4  |
| VIII | Figure S2 XAFS data at room and low temperatures .....                                               | 5  |
| IX   | Figure S3 Radial distribution functions in $C2/c$ , $C2/m$ , and $P2_1/c$ at ambient pressure .....  | 6  |
| X    | Figure S4 Calculated band gap versus pressure for $P2_1/c$ and $\alpha\text{-}P\bar{1}$ phases ..... | 7  |
| XI   | Figure S5 Total and projected DOS of the $P2_1/c$ structure at ambient pressure .....                | 8  |
| XII  | Figure S6 Total and projected DOS of the $\alpha\text{-}P\bar{1}$ structure at 10 GPa .....          | 9  |
| XIII | Figure S7 Total and projected DOS of the $\alpha'\text{-}P\bar{1}$ structure at 25 GPa .....         | 10 |
| XIV  | Figure S8 Comparison of $P2_1/c$ and $C2/m$ phases .....                                             | 11 |

---

\* gfabbris@anl.gov

## I. FURTHER DETAILS ON THE POWDER X-RAY DIFFRACTION ANALYSIS

High pressure powder x-ray diffraction was collected in angular dispersive mode using a MAR345 area detector. Representative raw data are shown in Fig. S1(a). The observed textured powder rings is a known limitation of high-pressure measurements performed in a diamond anvil cell, that occurs due to the small sample volume and thus poor powder averaging. Such texture, combined with the low structural symmetry of  $\text{Cu}_2\text{IrO}_3$ , prevents us from refining the atomic positions at high pressure.

Figure S1(b) displays the Rietveld refinement of  $P2_1/c$  phase at ambient pressure over the whole measured  $2\theta$  range. Figure S1(c)&(d) show Rietveld refinements of the  $P2_1/c$  (phase 1) and  $\alpha\text{-}P\bar{1}$  (phase 2) structures at high pressure. The atomic positions were fixed to those measured at ambient pressure for  $P2_1/c$  and to the theoretical values for  $\alpha\text{-}P\bar{1}$  (see Tables S2 & S3), and the background was modelled with an 3<sup>th</sup>/8<sup>th</sup>-order Chebyshev polynomial for ambient and high pressure, respectively. The presence of stacking faults was best modelled by assuming a complete mixing the Cu and Ir sites in the honeycomb plane. The lattice constants and wRs are reported in Table S1. The refinements are noticeably worse for the high pressure  $\alpha\text{-}P\bar{1}$  phase. Further work is in progress to understand the origin of this disagreement. As described in the main text, the theoretical dimerized Ir-Ir distance for this phase is larger than that seen by XAFS. However, attempts to fit the atomic positions in this phase have lead to inconclusive results, with multiple local minima configurations that display very different Ir-Ir distances.

Beyond 20 GPa, the phase obtained through the evolutionary algorithm is inconsistent with the experimental data [Table S4 and Fig. S1(d)]. However, as discussed in the manuscript, such disagreement might be related to the potential presence of multiple nearly degenerate ground states and/or the role of kinetics in this transition.

The phase transitions observed at room temperature are fully reversible as seen in Fig. S1(f) (a similar measurement was not performed at LT). This result is consistent with DFT calculations, as shown in Fig. 6(b) of the main manuscript.

## II. ADDITIONAL X-RAY ABSORPTION FINE STRUCTURE DATA

Figure S2 displays the  $\text{Cu}_2\text{IrO}_3$  Ir  $L_3$  XAFS data at room and low temperature. The phase 1-2 transition leads to changes in the  $\chi(R)$  [Fig. S2(a-c)&(l-n)], which are particularly distinct in the imaginary part [panels (c)&(n)]. The low structural symmetry of both phases 1 and 2 of  $\text{Cu}_2\text{IrO}_3$  leads to a large number of parameters that need to be constrained. In both  $P2_1/c$  and  $\alpha\text{-}P\bar{1}$  structures, we can split the most relevant scattering paths for XAFS into three groups: first neighbor Ir-O ( $R \sim 2$  Å,  $\text{IrO}_6$  octahedra), in-plane Ir-Ir and Ir-Cu ( $R \sim 3.15$  Å, forms the honeycomb lattice), and out-of-plane Ir-Cu ( $R \sim 3.4$  Å). The phase 1 XAFS is very well modelled using a single Debye-Waller factor and  $\Delta R$  parameters for each of these groups. We also add all multiple scattering paths with intensity larger than 2.5% of the strongest single scattering path. The phase 2 data, on the other hand, cannot be reproduced with this model. Instead, it requires that the three in-plane Ir-Ir paths be split into two groups, one short and two long distances, leading to the distances reported in Fig. 3(f) of the main text.

TABLE S1. Lattice constants extracted from the room temperature PXRD data using the atomic positions reported in Tables S2&S3. The 7.5 and 8.2 GPa data were best modelled by a combination of  $P2_1/c$  and  $\alpha\text{-}P\bar{1}$  structures. Data were modelled between 2.5-48 degrees at ambient pressure, and 3-21.2 degrees at high pressure.

| P (GPa)   | Space Group | wR (%) | $a$ (Å)   | $b$ (Å)    | $c$ (Å)   | $\alpha$ (°) | $\beta$ (°) | $\gamma$ (°) |
|-----------|-------------|--------|-----------|------------|-----------|--------------|-------------|--------------|
| $10^{-4}$ | $P2_1/c$    | 14.8   | 5.9689(2) | 9.33632(9) | 5.3894(2) | 90.0         | 107.7224(7) | 90.0         |
| 0.9       | $P2_1/c$    | 3.0    | 5.971(2)  | 9.3182(5)  | 5.380(2)  | 90.0         | 107.774(5)  | 90.0         |
| 3.3       | $P2_1/c$    | 3.6    | 5.966(2)  | 9.2397(6)  | 5.335(2)  | 90.0         | 107.659(5)  | 90.0         |
| 5.7       | $P2_1/c$    | 3.9    | 5.964(2)  | 9.1635(6)  | 5.292(2)  | 90.0         | 107.537(6)  | 90.0         |
| 6.7       | $P2_1/c$    | 4.1    | 5.964(2)  | 9.1350(7)  | 5.276(2)  | 90.0         | 107.504(6)  | 90.0         |
| 7.5       | $P2_1/c$    | 3.6    | 5.971(4)  | 9.152(1)   | 5.263(3)  | 90.0         | 107.594(9)  | 90.0         |
| 7.5       | $P\bar{1}$  | 3.6    | 5.968(3)  | 9.121(1)   | 5.193(3)  | 89.927(9)    | 107.67(1)   | 89.56(2)     |
| 8.2       | $P2_1/c$    | 4.2    | 5.976(5)  | 9.107(2)   | 5.241(4)  | 90.0         | 107.73(2)   | 90.0         |
| 8.2       | $P\bar{1}$  | 4.2    | 5.972(3)  | 9.139(1)   | 5.182(3)  | 89.918(8)    | 107.714(9)  | 89.562(12)   |
| 9.1       | $P\bar{1}$  | 5.2    | 5.975(3)  | 9.1101(7)  | 5.174(3)  | 89.930(8)    | 107.784(9)  | 89.698(14)   |
| 10.6      | $P\bar{1}$  | 5.1    | 5.979(3)  | 9.0764(6)  | 5.155(2)  | 89.979(7)    | 107.936(8)  | 89.687(13)   |
| 12.0      | $P\bar{1}$  | 5.1    | 5.981(3)  | 9.0428(6)  | 5.135(2)  | 89.981(7)    | 108.070(7)  | 89.654(12)   |
| 12.9      | $P\bar{1}$  | 5.1    | 5.983(3)  | 9.0195(6)  | 5.120(2)  | 89.966(7)    | 108.194(7)  | 89.635(12)   |

TABLE S2. Atomic positions of the  $P2_1/c$  phase of  $\text{Cu}_2\text{IrO}_3$  at 1 bar obtained from *ab-initio* calculations and Rietveld refinement. Monoclinic symmetry,  $P2_1/c$  (number 14) space group, and theoretical lattice constants  $a = 6.024$  Å,  $b = 9.485$  Å,  $c = 5.424$  Å, and  $\beta = 108.061^\circ$ . Experimental constants are reported in Table S1. Oxygen atomic positions were not experimentally refined due to poor sensitivity of 27 keV x-rays. The atomic sites 2d and 2a are constrained by symmetry.

| Atom | Site | x        |           | y        |           | z        |           | $U_{\text{iso}}$ |
|------|------|----------|-----------|----------|-----------|----------|-----------|------------------|
|      |      | Th.      | Exp.      | Th.      | Exp.      | Th.      | Exp.      |                  |
| Ir   | 4e   | 0.508405 | 0.5056(3) | 0.833333 | 0.8341(1) | 0.992092 | 1.0010(4) | 0.0059(1)        |
| Ir   | 2d   | -        | 0.5       | -        | 0.5       | -        | 0         | 0.0059(1)        |
| Cu   | 2d   | 0.5      | 0.5       | 0.5      | 0.5       | 0        | 0         | 0.0074(3)        |
| Cu   | 4e   | -        | 0.5056(3) | -        | 0.8341(1) | -        | 1.0010(4) | 0.0074(3)        |
| Cu   | 4e   | 0.985454 | 1.0016(7) | 0.178180 | 0.1845(3) | 0.518739 | 0.5184(8) | 0.0074(3)        |
| Cu   | 2a   | 0.0      | 0.0       | 0.5      | 0.5       | 0.5      | 0.5       | 0.0074(3)        |
| O    | 4e   | 0.326050 | -         | 0.505811 | -         | 0.607166 | -         | 0.0074(3)        |
| O    | 4e   | 0.306999 | -         | 0.181513 | -         | 0.626691 | -         | 0.0074(3)        |
| O    | 4e   | 0.662262 | -         | 0.162762 | -         | 0.404779 | -         | 0.0074(3)        |

TABLE S3. Atomic positions of the  $\alpha$ - $P\bar{1}$  phase of  $\text{Cu}_2\text{IrO}_3$  at 10 GPa obtained from *ab-initio* calculations. Triclinic symmetry,  $P\bar{1}$  (number 2) space group,  $a = 6.060$  Å,  $b = 9.191$  Å,  $c = 5.121$  Å,  $\alpha = 92.949^\circ$ ,  $\beta = 107.315^\circ$ , and  $\gamma = 88.112^\circ$ .

| Atom | Site | x        | y        | z        |
|------|------|----------|----------|----------|
| Ir   | 2i   | 0.007629 | 0.668472 | 0.004961 |
| Ir   | 2i   | 0.009223 | 0.830908 | 0.489701 |
| Cu   | 1a   | 0.0      | 0.0      | 0.0      |
| Cu   | 1e   | 0.5      | 0.5      | 0.0      |
| Cu   | 1f   | 0.5      | 0.0      | 0.5      |
| Cu   | 2i   | 0.518592 | 0.675824 | 0.490059 |
| Cu   | 1g   | 0.0      | 0.5      | 0.5      |
| Cu   | 2i   | 0.494368 | 0.173018 | 0.009954 |
| O    | 2i   | 0.179614 | 0.001915 | 0.397992 |
| O    | 2i   | 0.207359 | 0.664760 | 0.399462 |
| O    | 2i   | 0.834157 | 0.668971 | 0.598797 |
| O    | 2i   | 0.820081 | 0.506651 | 0.100108 |
| O    | 2i   | 0.807386 | 0.181780 | 0.114842 |
| O    | 2i   | 0.180767 | 0.154309 | 0.913190 |

TABLE S4. Atomic positions of the  $\alpha'$ - $P\bar{1}$  phase of  $\text{Cu}_2\text{IrO}_3$  at 25 GPa obtained from *ab-initio* calculations. Triclinic symmetry,  $P\bar{1}$  (number 2) space group,  $a = 4.973$  Å,  $b = 5.231$  Å,  $c = 5.317$  Å,  $\alpha = 61.052^\circ$ ,  $\beta = 68.432^\circ$ , and  $\gamma = 76.498^\circ$ .

| Atom | Site | x        | y        | z        |
|------|------|----------|----------|----------|
| Ir   | 2i   | 0.988709 | 0.337225 | 0.332595 |
| Cu   | 1a   | 0.0      | 0.0      | 0.0      |
| Cu   | 1f   | 0.5      | 0.0      | 0.5      |
| Cu   | 2i   | 0.502033 | 0.332354 | 0.831965 |
| O    | 2i   | 0.218709 | 0.287930 | 0.610875 |
| O    | 2i   | 0.224212 | 0.655425 | 0.941071 |
| O    | 2i   | 0.744576 | 0.010770 | 0.707418 |

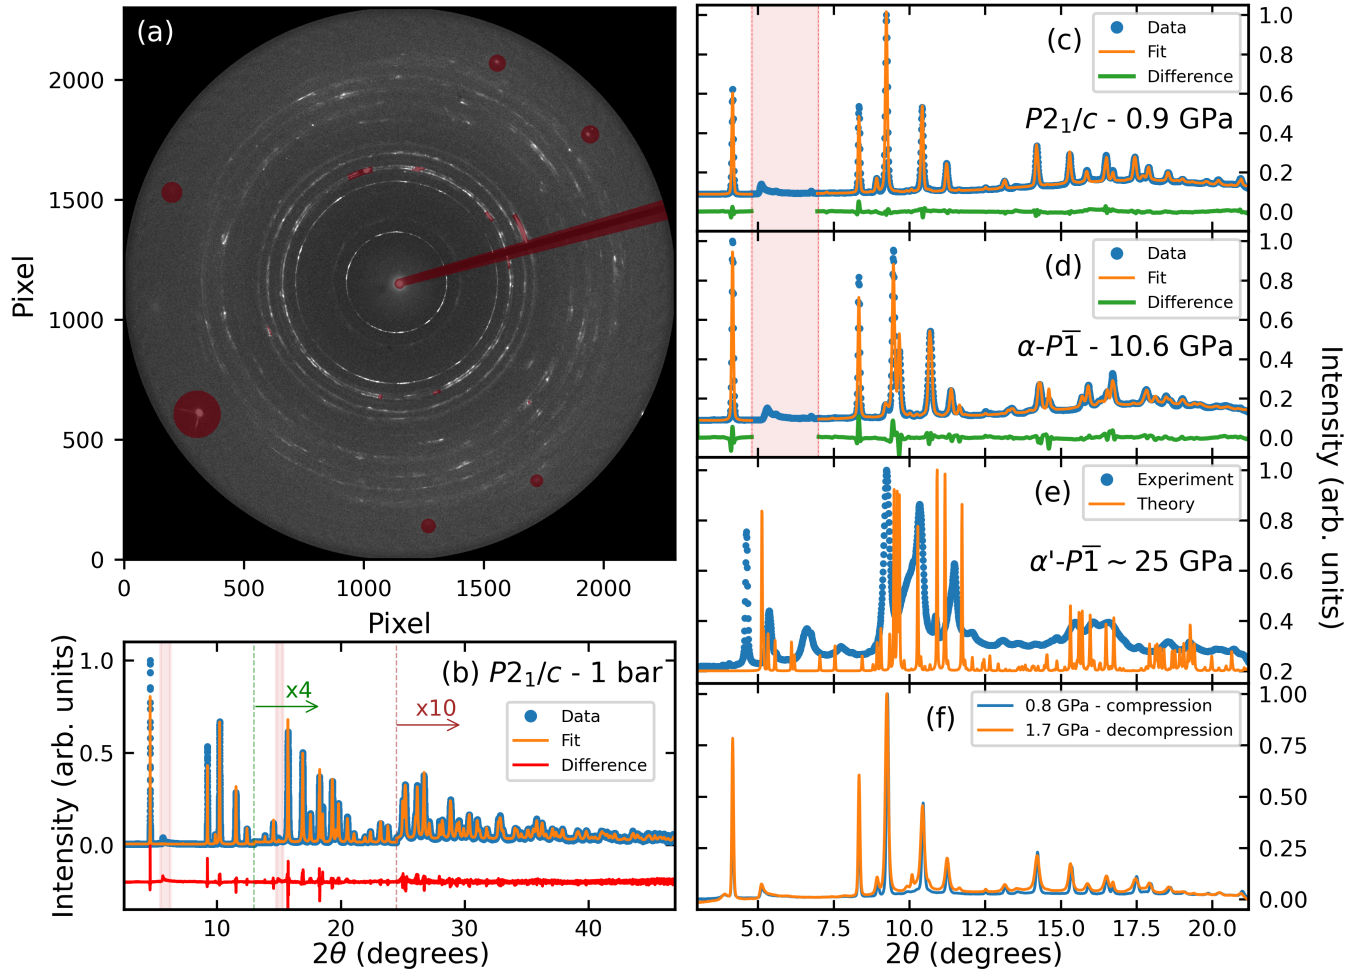

FIG. S1. Cu<sub>2</sub>IrO<sub>3</sub> powder x-ray diffraction data at room temperature. (a) 2D raw image. Spurious single crystal Bragg peaks were removed using a mask shown in red. (b-d) Rietveld refinements of the 1 bar, 0.9 GPa and 10.6 GPa data, respectively. (e) The experimental data at 25.5 GPa is compared to the theoretically predicted phase at 25 GPa. (f) Low pressure data measured during compression and decompression (after reaching 40 GPa).

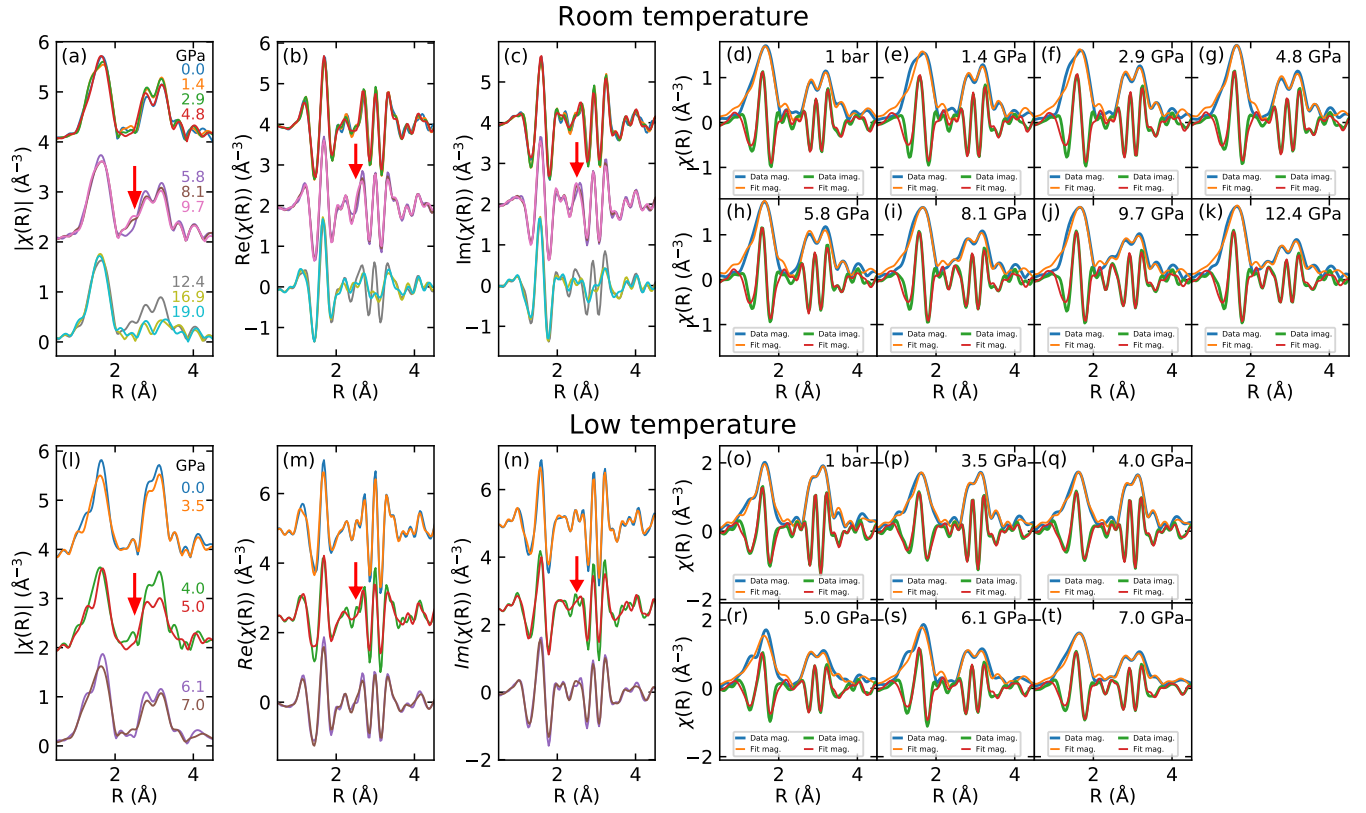

FIG. S2.  $\text{Cu}_2\text{IrO}_3$  Ir  $L_3$  XAFS as a function of pressure at room temperature (top panels) and 15 K (bottom panels). For both temperatures, a spectral weight change is observed at a similar  $R$  (red arrows in panels (a-c)&(l-n)). These changes are well reproduced at both temperatures by splitting the Ir-Ir distances (panels (d-k)&(o-t)).

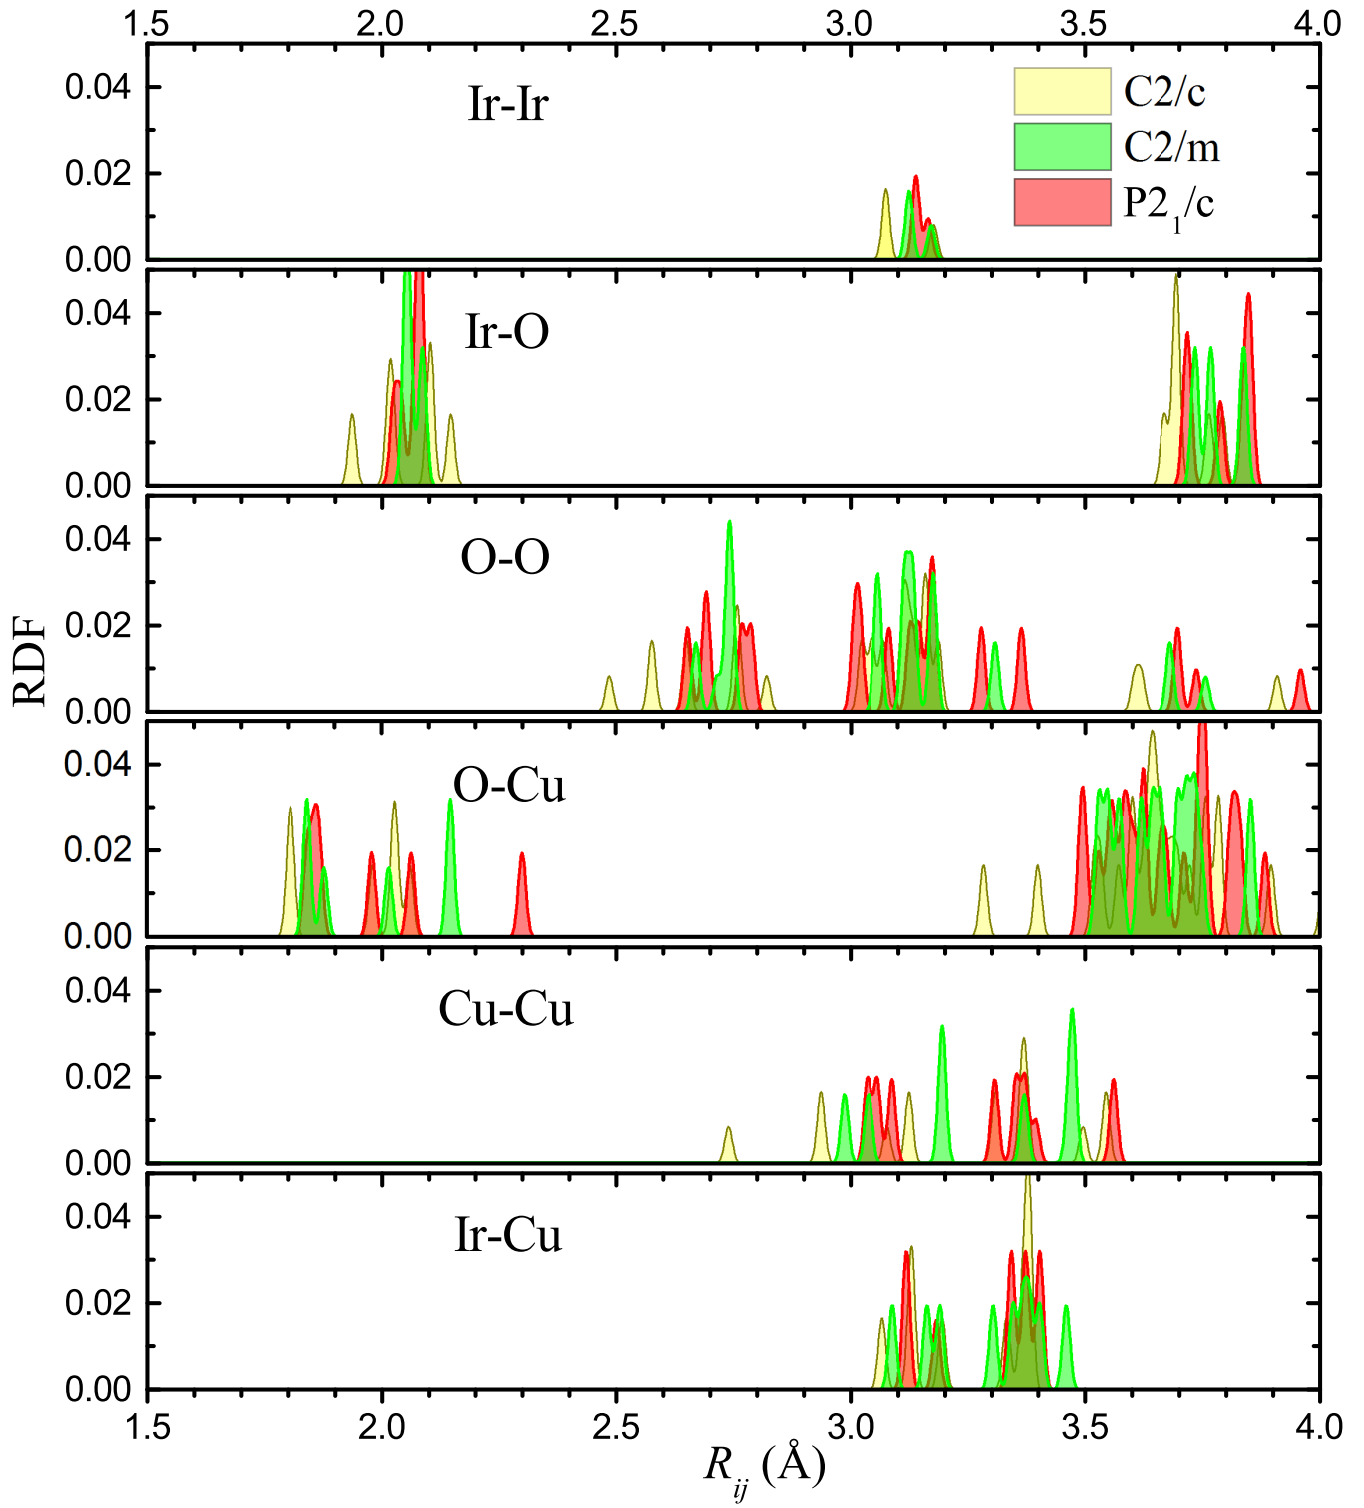

FIG. S3. Radial distribution functions for the experimental  $C2/c$  solution at ambient pressure and the proposed  $C2/m$  and  $P2_1/c$  phases optimized with DFT+U+SO at 0 GPa. While bond lengths in the GGA are typically overestimated by 1-2%, some of the Cu-Cu distances in  $C2/c$  are unphysically short.

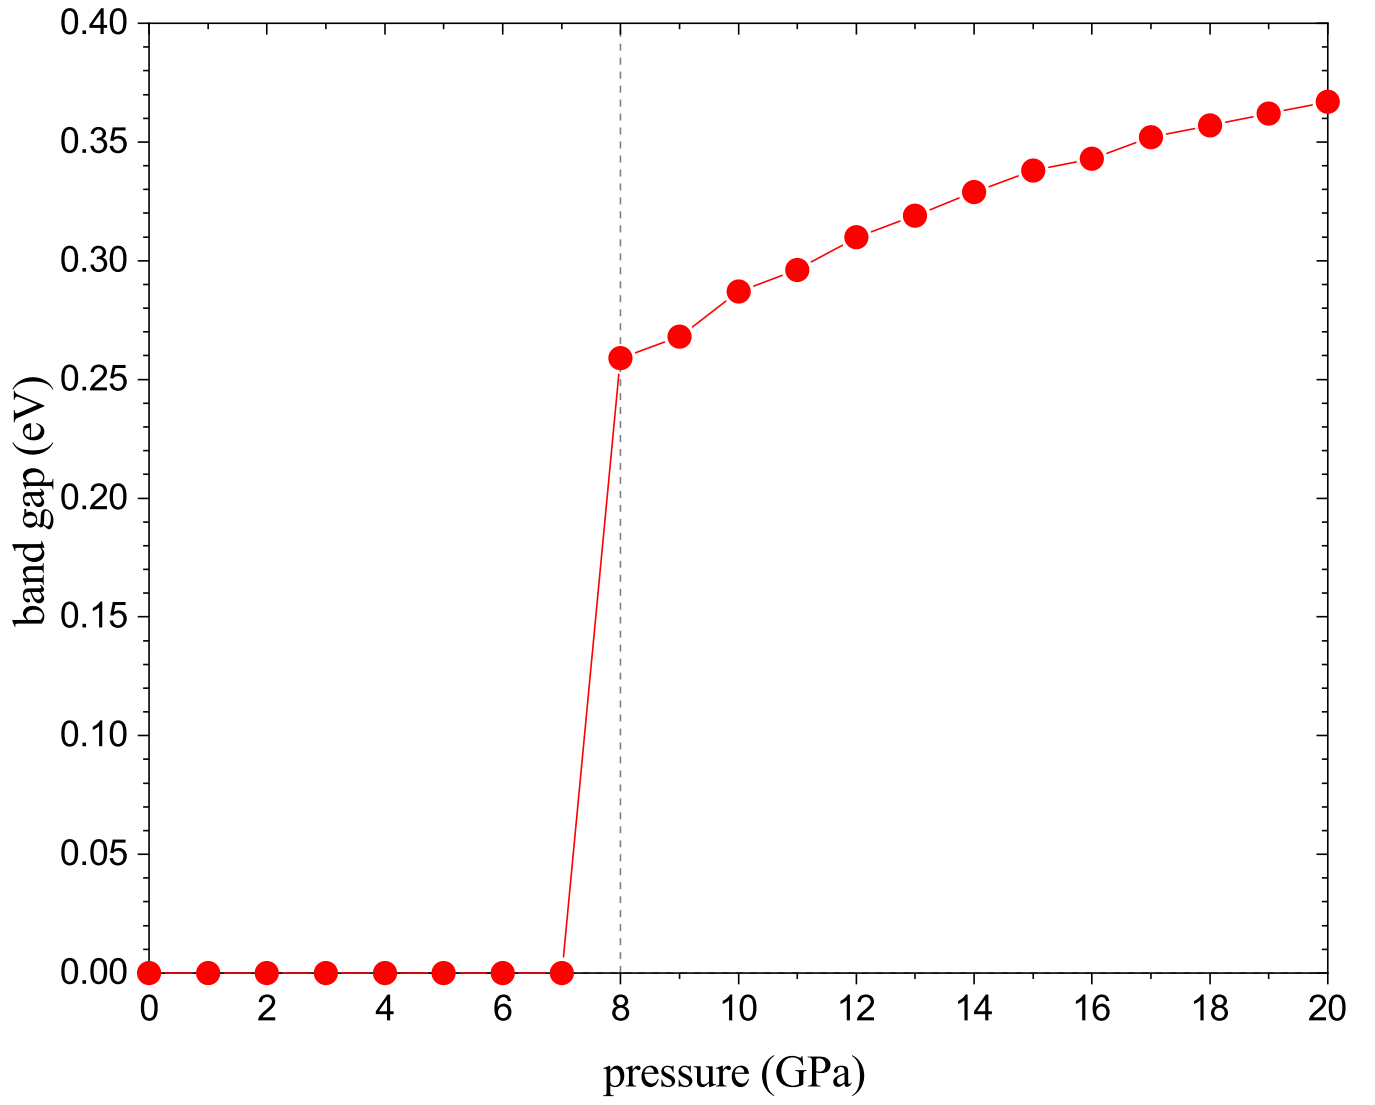

FIG. S4. Band gap in  $P2_1/c$  (below 8 GPa) and  $\alpha\text{-}P\bar{1}$  (above 8 GPa) as a function of the applied pressure calculated at the DFT+U+SO level. Note the correlation between the band gap and the Ir-Ir bond dimerization value (Fig. 6 of the main manuscript) in the considered pressure range.

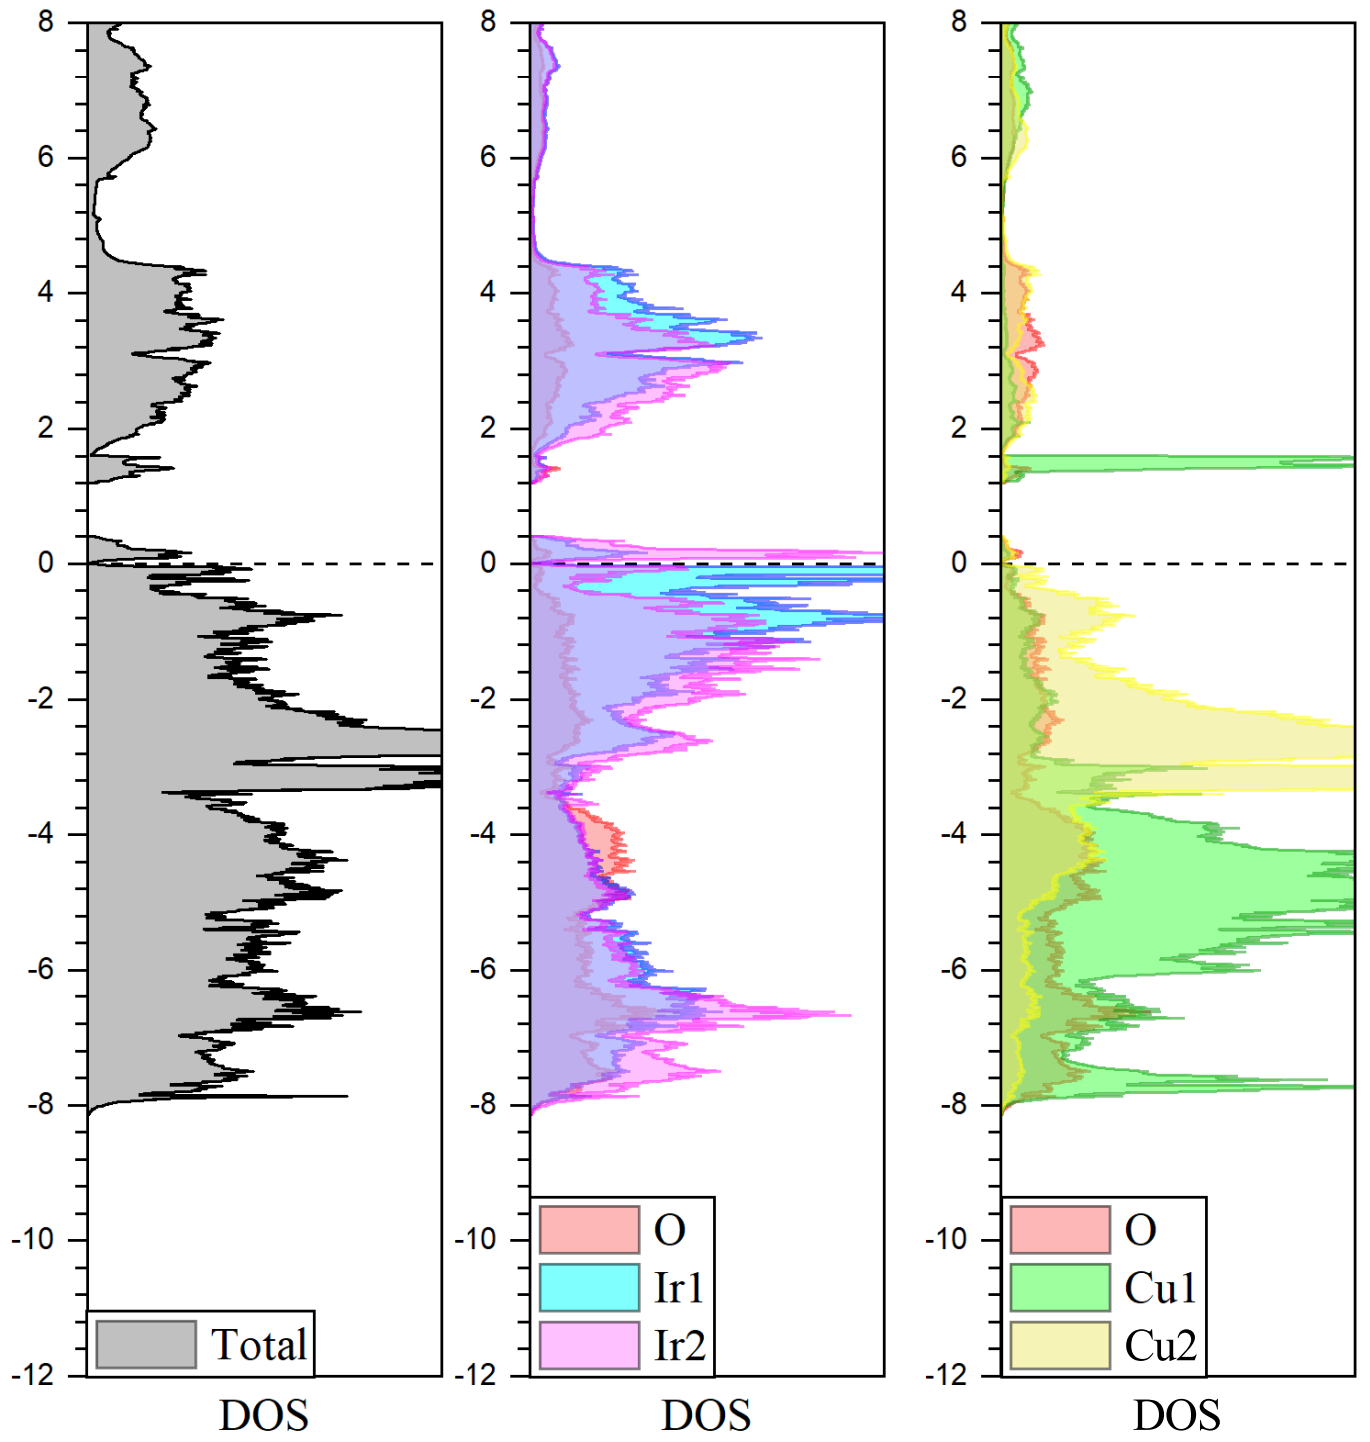

FIG. S5. DOS of the  $P2_1/c$  structure at 0 GPa projected onto individual atoms. Cu1/Cu2 refers to the combined DOS of all Cu sites in/out-of the honeycomb planes, respectively.

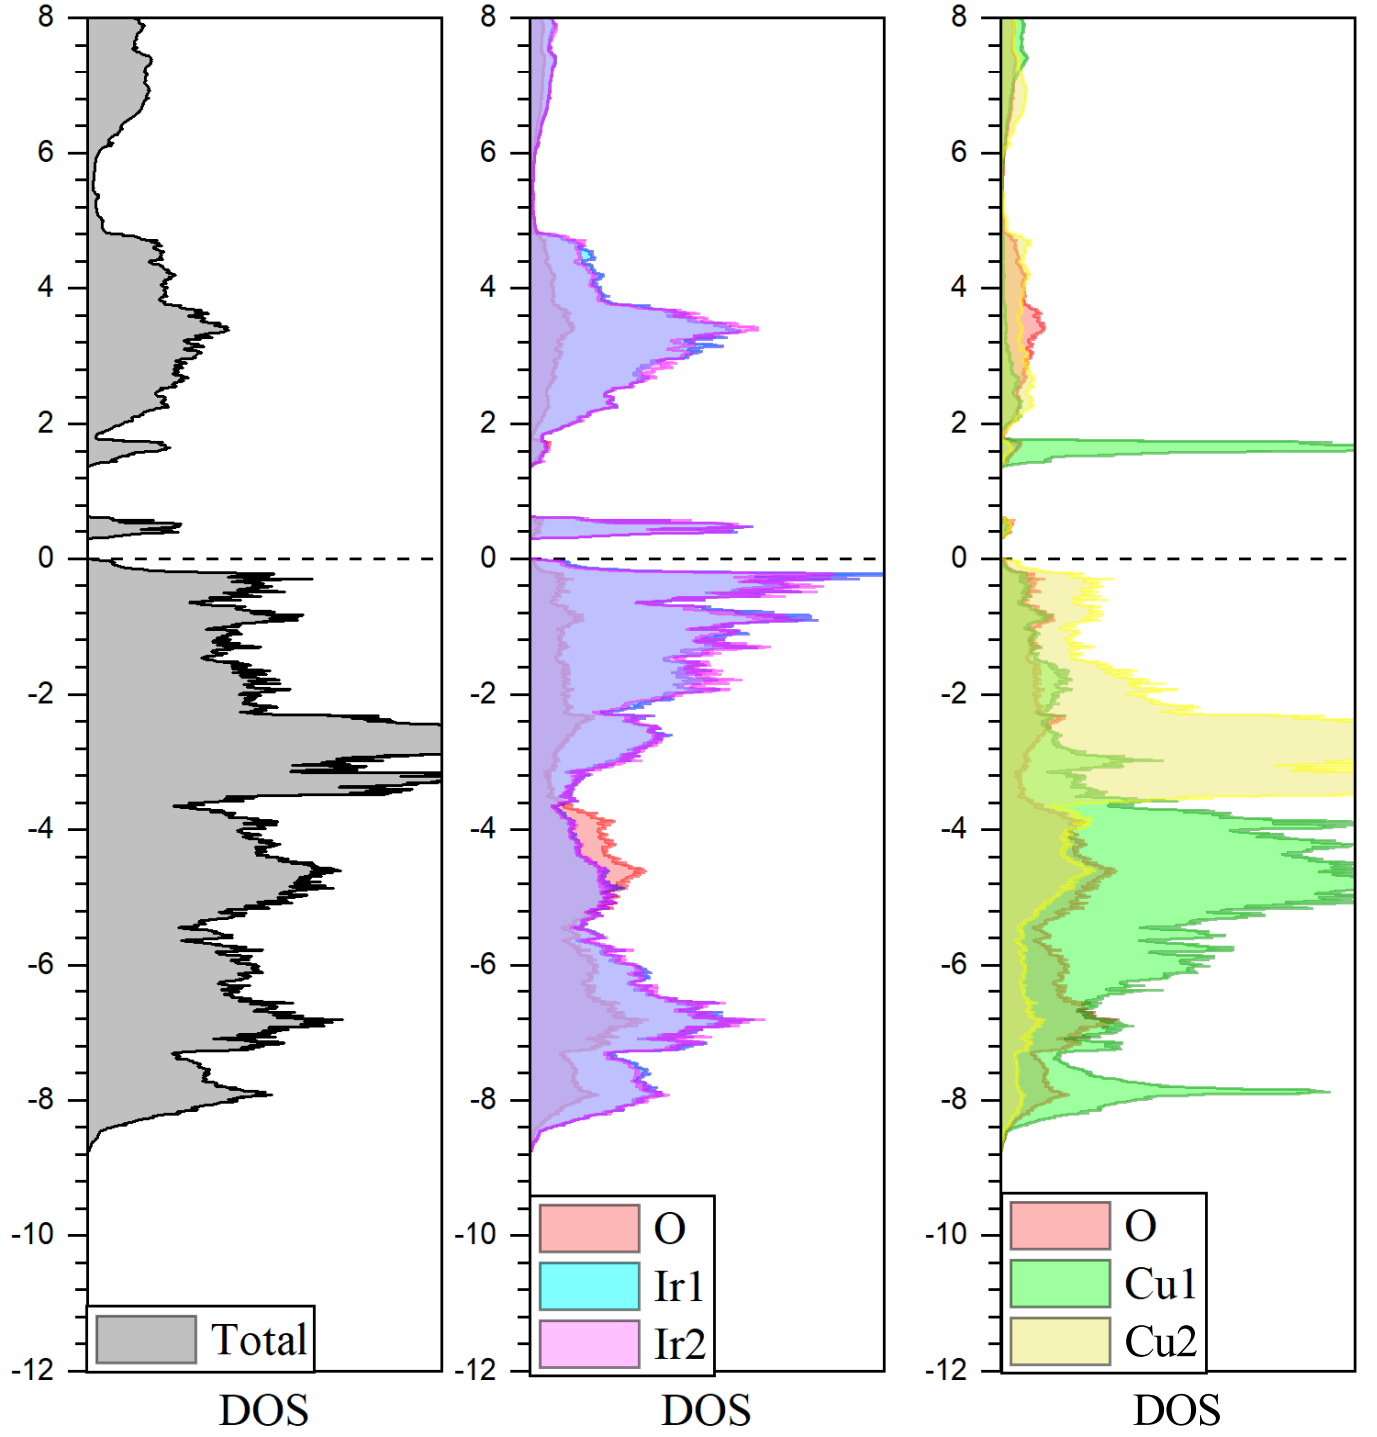

FIG. S6. Total and projected DOS of the  $\alpha\text{-P}\bar{1}$  structure at 10 GPa. Cu1/Cu2 refers to the combined DOS of all Cu sites in/out-of the honeycomb planes, respectively.

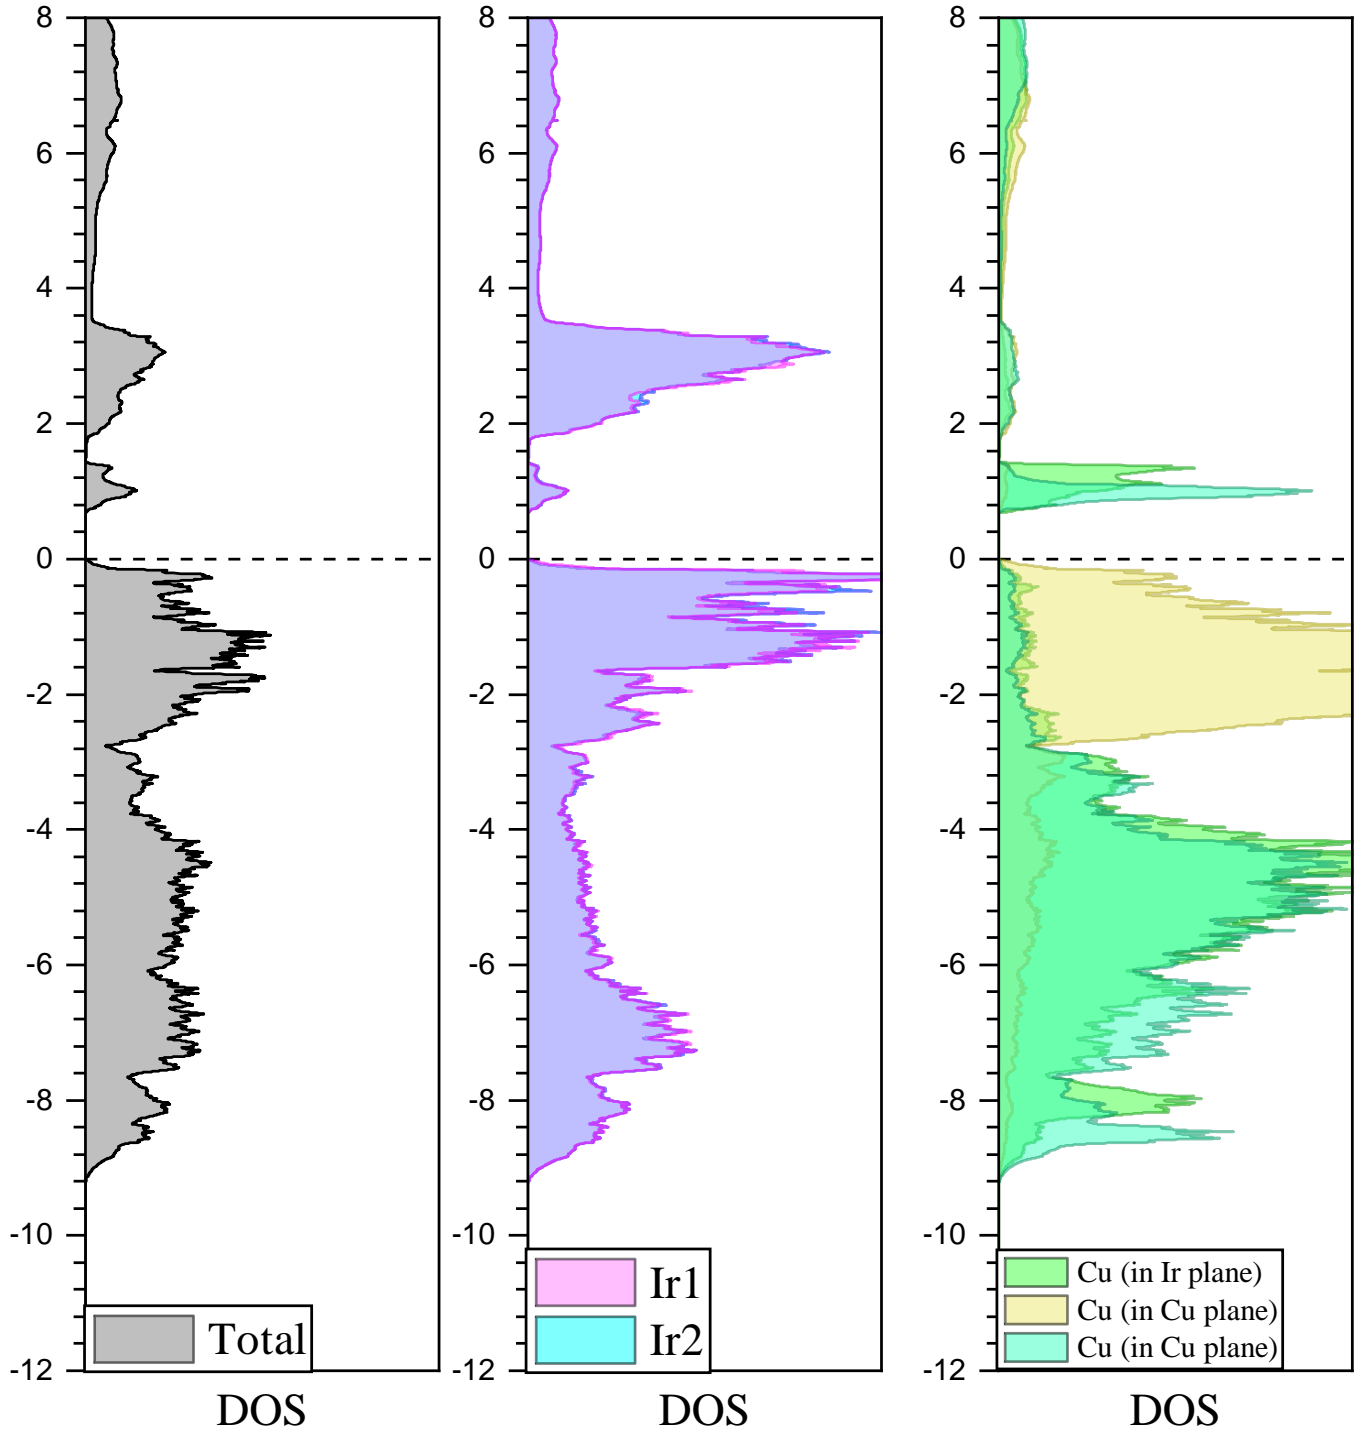

FIG. S7. Total and projected DOS of the  $\alpha'$ -P1 structure at 25 GPa.

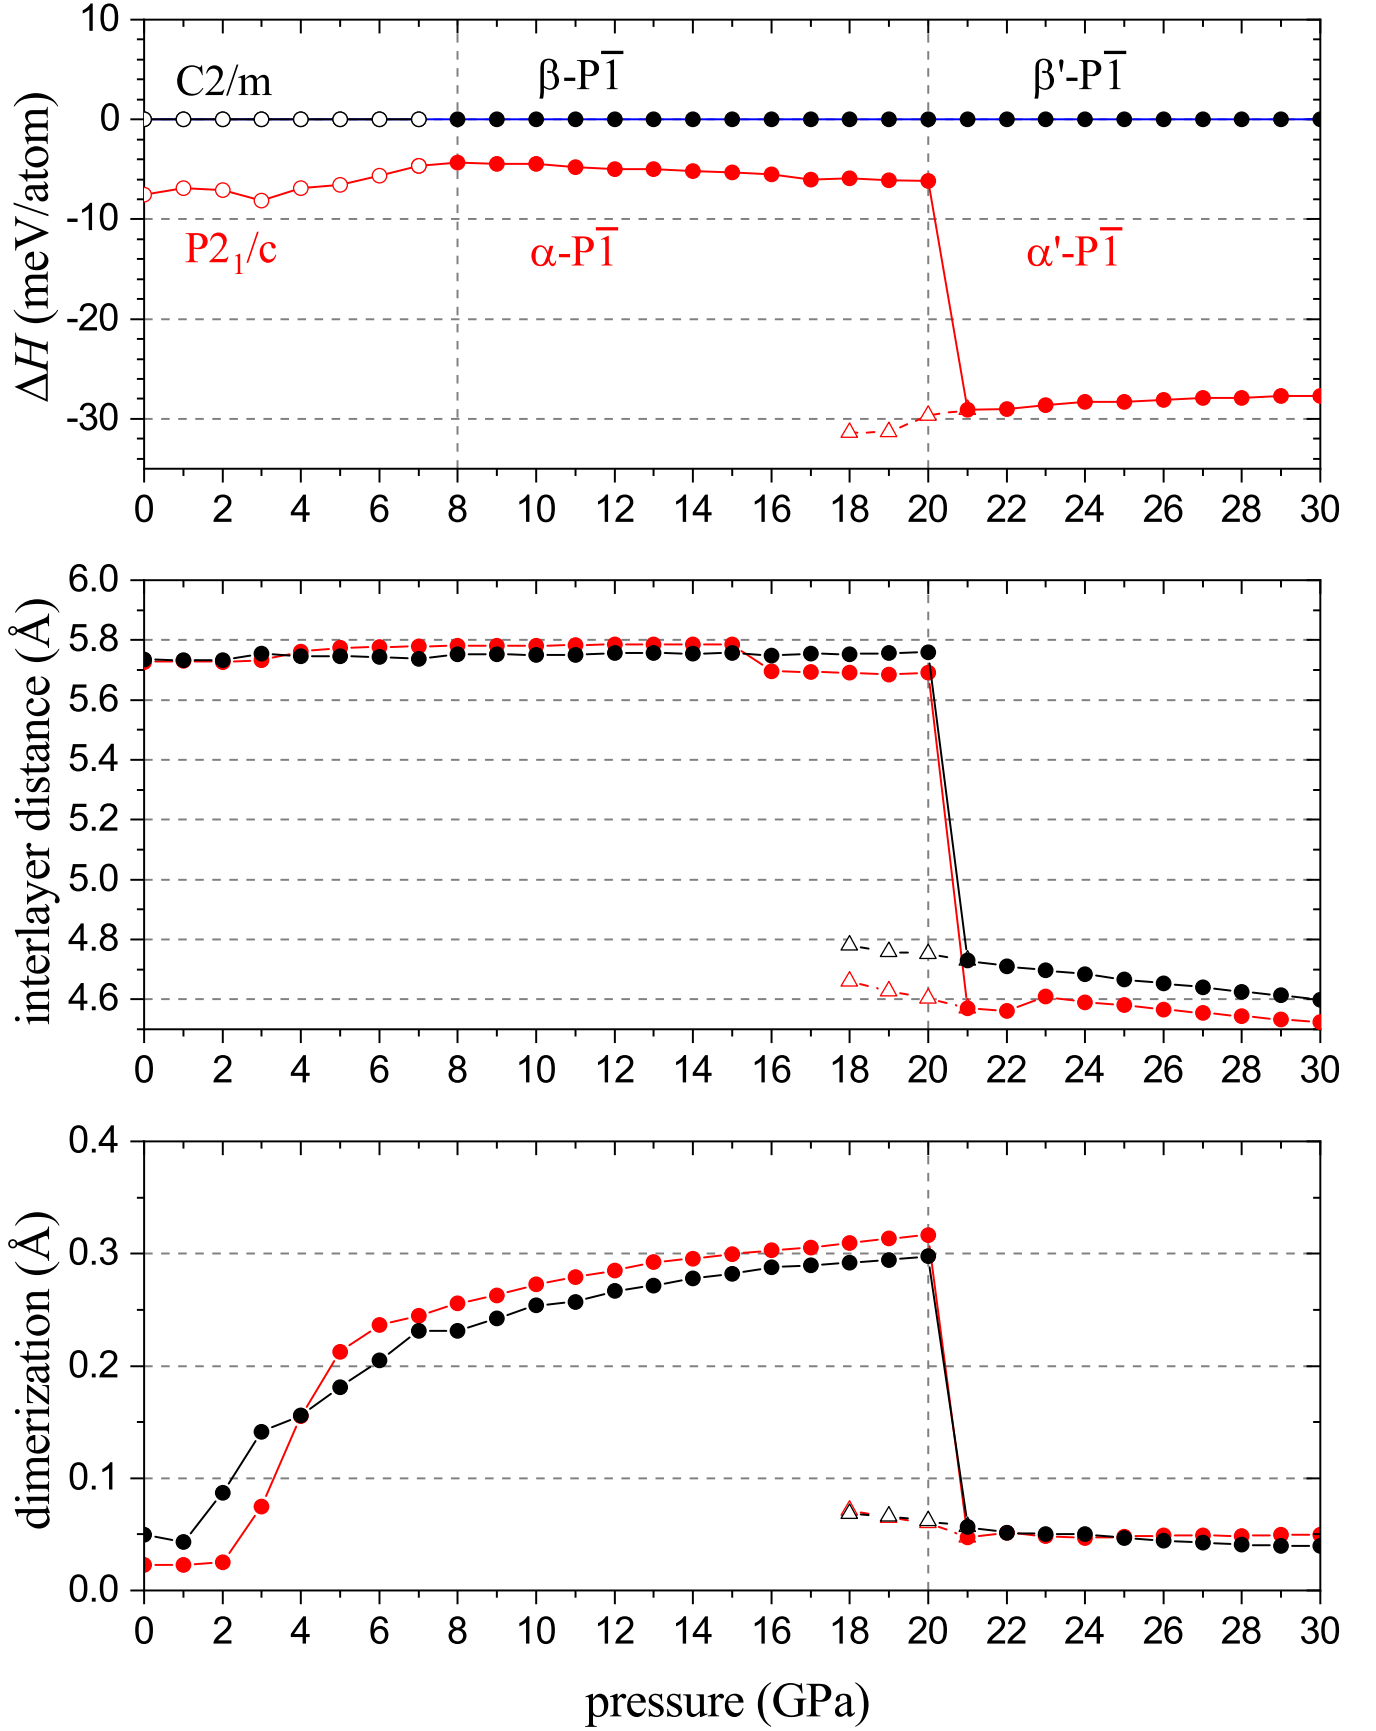

FIG. S8. Relative enthalpy (top), interlayer distance (middle), Ir-Ir dimerization (bottom) as a function of pressure for fully optimized competing structures of  $\text{Cu}_2\text{IrO}_3$ . The interlayer distance is calculated as the vertical spacing between nearest Ir-Cu layers. The dimerization is taken as the difference between the longest and the shortest Ir-Ir bonds connecting an Ir atom to its three nearest neighbors in the honeycomb lattice. The proposed  $P2_1/c$ ,  $\alpha-P\bar{1}$ , and  $\alpha'-P\bar{1}$  are found to be the lowest-enthalpy phases in the 0-30 GPa pressure range.
